# Supplementary material for: Uncertainty Quantification of First Principles Computational Phase Diagram Predictions of Li-Si System Via Bayesian Sampling
Source: arXiv:2003.13393 source file (2020-02-23)
Supplement: Supplementary file 1 [file SI.pdf]

# Supplimentary Information for: Uncertainty Quantification of First Principles Computational Phase Diagram Predictions of Li-Si System Via Bayesian Sampling

Ying Yuan,[1] Gregory Houchins,[2] Pin-Wen Guan,[3] and Venkatasubramanian Viswanathan[4,5,3]

[1] *Department of Materials Science and Engineering, Carnegie Mellon University, Pittsburgh, Pennsylvania 15213, USA*

[2] *Department of Physics, Carnegie Mellon University,Pittsburgh, Pennsylvania 15213, USA*

[3] *Department of Mechanical Engineering, Carnegie Mellon University, Pittsburgh, Pennsylvania 15213, USA*

[4] *Department of Materials Science and Engineering, Carnegie Mellon University, Pittsburgh, Pennsylvania 15213, USA*

[5] *Department of Physics, Carnegie Mellon University, Pittsburgh, Pennsylvania 15213, USA*

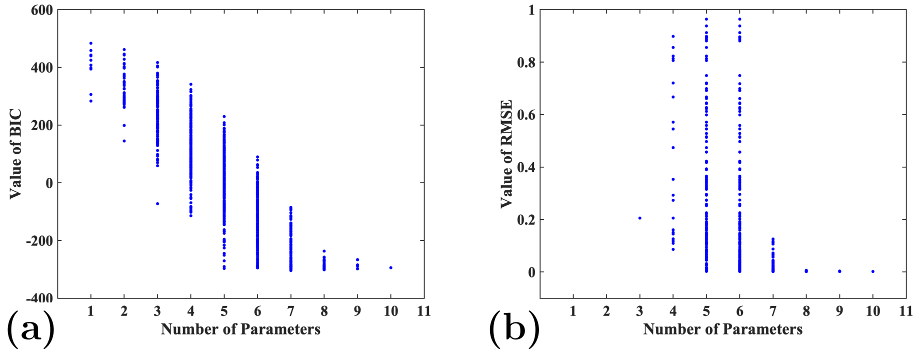


FIG. S1. (a) BIC model selection results and (b) RMSE results for solid phase Li.

## I. COMPUTATIONAL DETAILS

First, we use Quantum Espresso (QE) to relax cells of Li-Si system. Since the product of the number of k points and the lattice parameter (angstrom) in each dimension should be larger than a certain threshold, which depends on the system. Usually, for insulator or semiconductor, it can be as low as 20; for metal, it should be larger than 30. According this, we choose k-points for Li, Si, $Li_{15}Si_4$, $Li_{22}Si_5$, $Li_{21}Si_5$, $Li_{13}Si_4$, LiSi, $Li_7Si_2$, $Li_{12}Si_7$, $Li_{17}Si_4$, $Li_{4.11}Si$, $Li_7Si_3$ as (9 9 9), (4 4 4), (3 3 3), (2 2 2), (2 2 2), (3 2 6), (3 3 5), (3 2 6), (4 2 2), (2 2 2), (6 1 2), (4 4 2). The etot_conv_thr is 1.0E-4, the forc_conv_thr is 1.0E-3. The ecutwfc is 78.3, the ecutrho is 355. We also use Li.pbe-s-kjpaw_psl.0.2.1.UPF and Si.pbe-n-kjpaw_psl.0.1.UPF from database http://www.quantum-espresso.org/pseudopotentials. In this work, we finished the calculation without the use of Hubbard U.

All density functional calculations were performed using the Projector Augmented Wave-function as implement in real space within the GPAW software with a grid spacing of 0.16 Å, the K-points for per cell is the same with the value we take in QE calculation.

Using the fitted properties of the equation of state, a Debye-Grunessen theory analysis[1] was used to incorporate vibrational properties and predict the Gibbs free energy as a function of temperature. This process was repeated for the ensemble of 2000 non-self consistent exchange-correlation functionals within the BEEF-vdW model space framework. But not all of the 2000 functionals provided sufficient energy-volume data to fit an equation of state, only 1385 out of 2000 functionals are successful.

TABLE S1. The BIC model selection results of Li-Si system in temperature range 200K-450K. The complexity of model structure of Gibbs energy function is 10.

| phase | a | b | c | d | e | f | g | h | i | j |
|---|---|---|---|---|---|---|---|---|---|---|
| Li | -24422.538 | -24.530 | 0 | -0.031 | 214251.997 | 0 | -5.110e-18 | 0 | 7.495e-09 | 4340.672 |
| Si | -2894.975 | 166.575 | -27.765 | 0 | 41636.534 | 0 | 0 | 0 | 0 | -1214.162 |
| $Li_{15}Si_4$ | -443626.371 | 3468.794 | -570.180 | 0 | 369763.869 | 0 | 0 | 0 | -7.873e-09 | -33589.971 |
| $Li_{22}Si_5$ | -469584.427 | 5524.736 | -898.039 | 0.093 | 0 | -5.663e-05 | 0 | 0 | 0 | -64520.925 |
| $Li_{21}Si_5$ | -512335.342 | 5330.885 | -865.680 | 0.099 | 0 | -5.051e-05 | 0 | 0 | 0 | -62637.749 |
| $Li_{13}Si_4$ | -219702.247 | 3926.697 | -597.984 | 0 | -1020268.645 | 0 | -1.477e-17 | 0 | 0 | -72271.715 |
| LiSi | -40324.485 | -80.406 | 20.630 | -0.222 | 0 | 0.0002 | 1.582e-17 | 0 | -8.768e-08 | 0 |
| $Li_7Si_2$ | 0 | 2895.664 | -439.875 | 0.153 | -1291940.707 | -5.012e-05 | 0 | 0 | 0 | -60805.280 |
| $Li_2Si$ | -47584.250 | 590.723 | -92.001 | -0.004 | 0 | 0 | 0 | 0 | 0 | -8436.189 |
| $Li_{12}Si_7$ | 0 | 7046.047 | -1083.820 | 0.653 | -3026346.993 | -0.0003 | 0 | 0 | 7.160e-08 | -143899.261 |
| $Li_{17}Si_4$ | -417056.207 | 4309.137 | -699.234 | 0.077 | 0 | -4.134e-05 | 0 | 0 | 0 | -50826.567 |
| $Li_{4.11}Si$ | -186712.509 | 0 | 11.547 | -0.508 | 0 | 0.0005 | 6.223e-17 | 0 | -2.525e-07 | 0 |
| $Li_7Si_3$ | -232109.429 | 1995.133 | -322.816 | 0.016 | 0 | 0 | 0 | 0 | -6.960e-09 | -23679.865 |

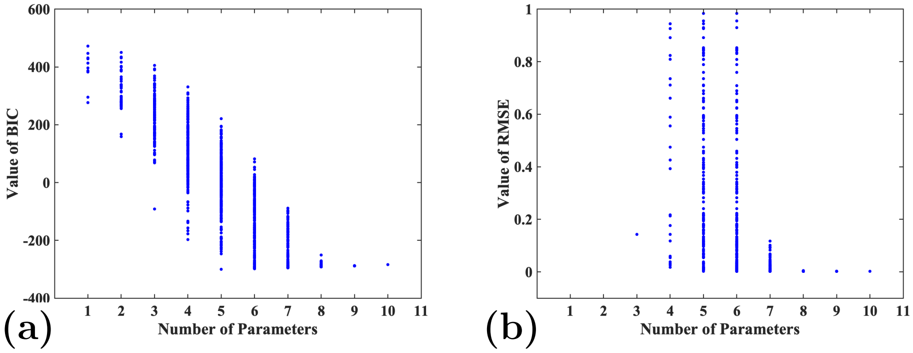


FIG. S2. (a) BIC model selection results and (b) RMSE results for solid phase Si.

## II. BIC MODEL SELECTION AND RESULTS

The BIC model selection results and RMSE results of other solid phases are shown in Figure S1-Figure S12.

Figure S13 shows the standard deviation of voltage at each x for the BEEF ensemble.

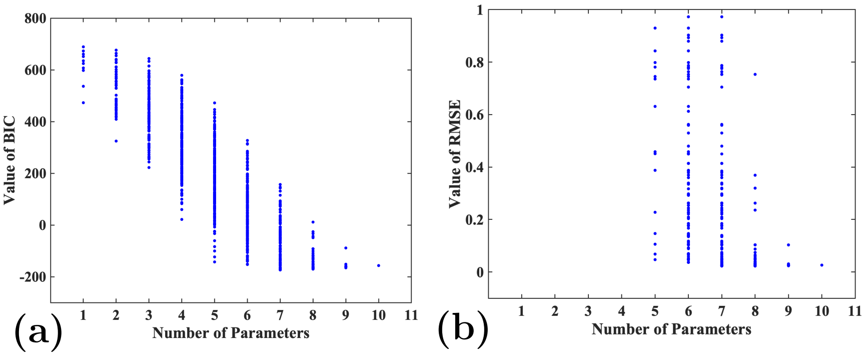


FIG. S3. (a) BIC model selection results and (b) RMSE results for solid phase $Li_{12}Si_7$.

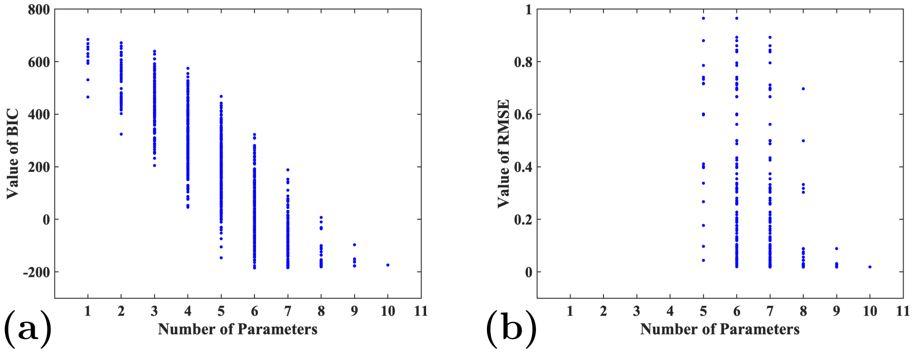


FIG. S4. (a) BIC model selection results and (b) RMSE results for solid phase $Li_{13}Si_4$.

With the filling fraction x increasing, the standard deviation of voltage changes, which agrees well with the voltage prediction.

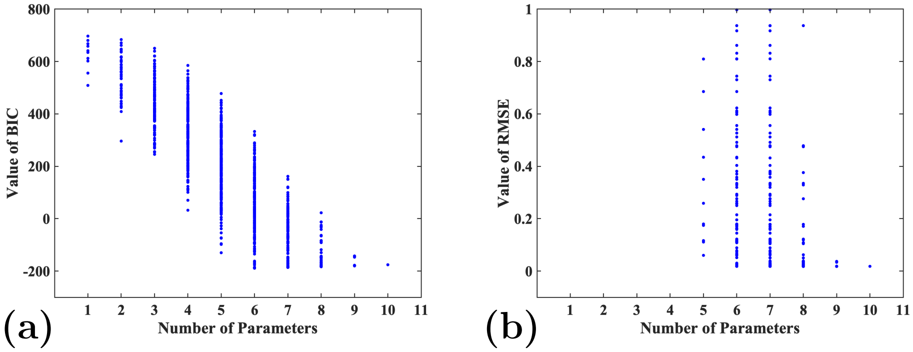


FIG. S5. (a) BIC model selection results and (b) RMSE results for solid phase $Li_{17}Si_4$.

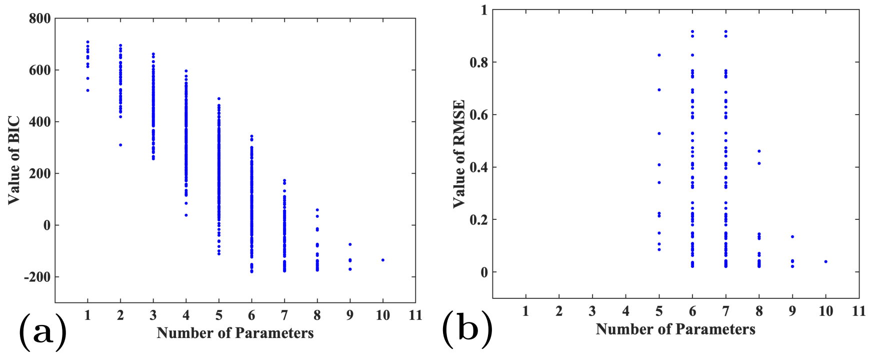


FIG. S6. (a) BIC model selection results and (b) RMSE results for solid phase $Li_{21}Si_5$.

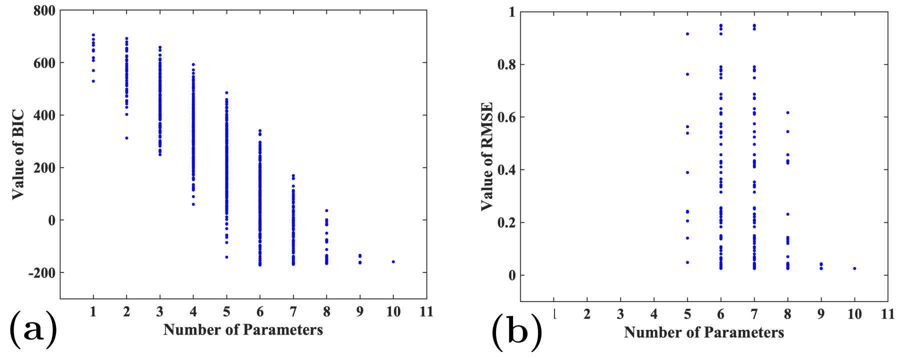


FIG. S7. (a) BIC model selection results and (b) RMSE results for solid phase $Li_{22}Si_5$.

## III. DERIVATION OF EQUILIBRIUM POTENTIAL

The potential for phase transformation from $Li_{x_1}Si$ to $Li_{x_2}Si$ is derived specifically here.

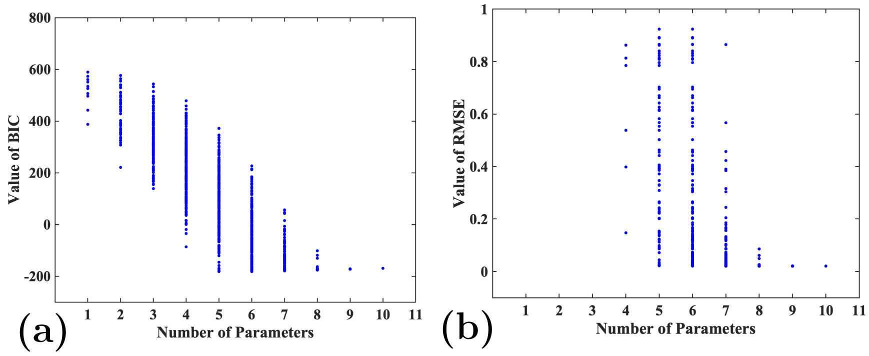


FIG. S8. (a) BIC model selection results and (b) RMSE results for solid phase $Li_2Si$.

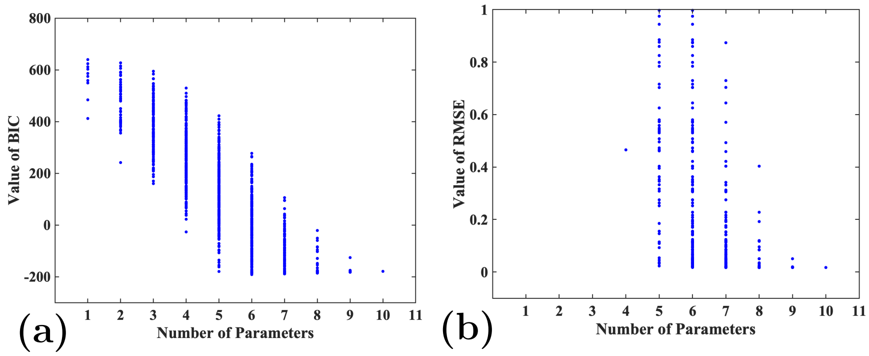


FIG. S9. (a) BIC model selection results and (b) RMSE results for solid phase $Li_{4.11}Si$.

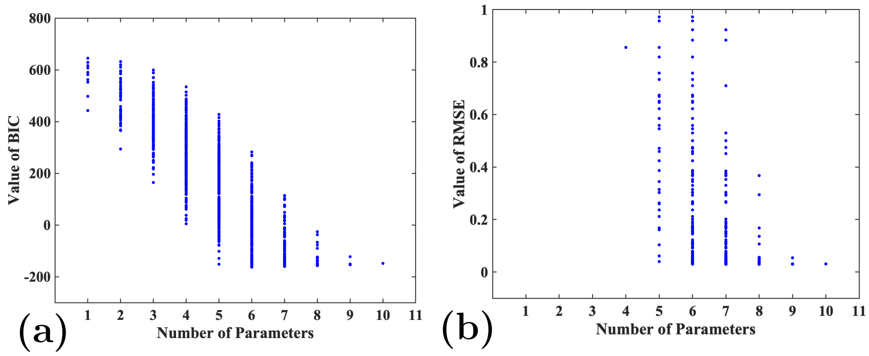


FIG. S10. (a) BIC model selection results and (b) RMSE results for solid phase $Li_7Si_2$.

The electrochemical lithiumcoupled ion transfer reaction with silicon is given by:

$$Li_{x_1}Si + (x_2 - x_1)(Li^+ + e^-) \rightleftharpoons Li_{x_2}Si \tag{1}$$

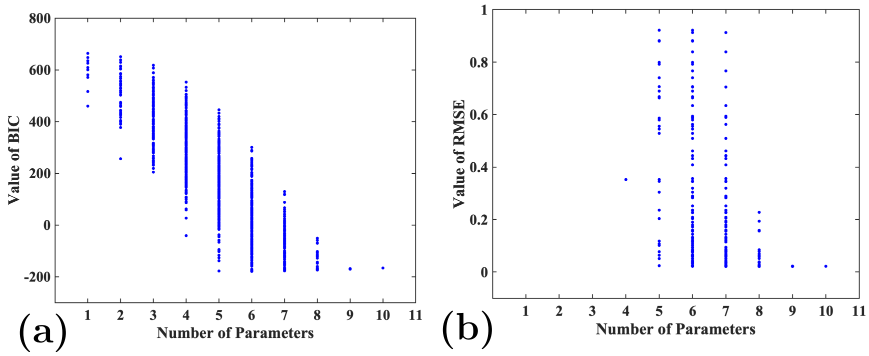


FIG. S11. (a) BIC model selection results and (b) RMSE results for solid phase $Li_7Si_3$.

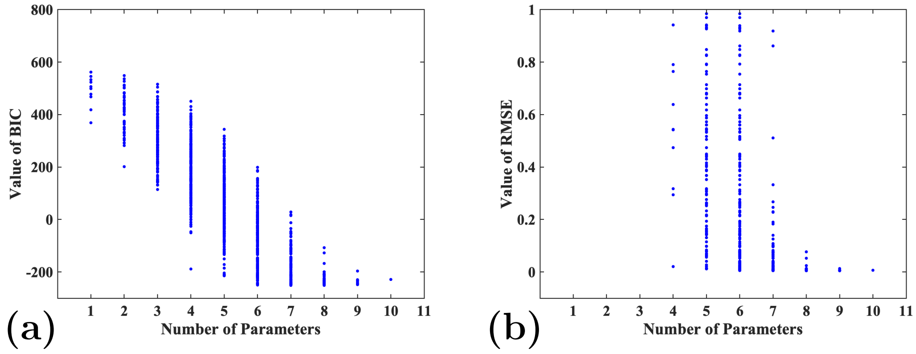


FIG. S12. (a) BIC model selection results and (b) RMSE results for solid phase LiSi.

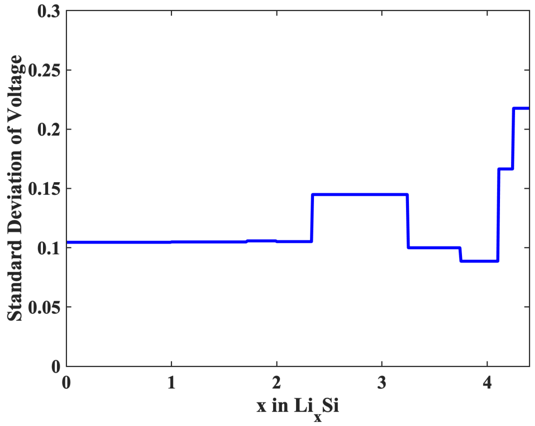


FIG. S13. The standard deviation of voltage of 1385 BEEF functionals of an ensemble at each filling fraction x.

The Gibbs free energy change associated with this process given by:

$$\begin{aligned} 0 &= G_{Li_{x_2}Si} - G_{Li_{x_1}Si} - (x_2 - x_1)(G_{Li^+} + G_{e^-}) \\ 0 &= G_{Li_{x_2}Si} - G_{Li_{x_1}Si} - (x_2 - x_1)(G_{Li_{(s)}} - eU_{Li/Li^+}) \\ (x_2 - x_1)eU_{Li/Li^+} &= -(G_{Li_{x_2}Si} - G_{Li_{x_1}Si} - (x_2 - x_1)G_{Li_{(s)}}) \\ U_{Li/Li^+} &= \frac{-1}{e(x_2 - x_1)}(G_{Li_{x_2}Si} - G_{Li_{x_1}Si} - (x_2 - x_1)G_{Li_{(s)}}) \end{aligned}$$

## REFERENCES

[1]Moruzzi, V. L., Janak, J. F. & Schwarz, K. Calculated thermal properties of metals. *Phys. Rev. B* **37**, 790–799 (1988).
